# Supplementary material for: Featured Team Automata
Source: arXiv:2108.01784 source file (2021-08-03)
Supplement: Supplementary file 1 [file appendix.tex]

% !TEX root=team.tex

\section{Synchronization types (with variability)}
%\guille{ongoing, need to do more checks}

===Guille: ongoing, need to do more checks\\

\myparagraph{Synchronization types with variability:} 
%\guille{notation to be decided}

===Guille:
notation to be decided\\

\begin{itemize}
	\item $\stype:\com \to (\sem{\mi{fm}}_F \to (\kw{snd},\kw{rcv}))$
\end{itemize}
%\guille{$\sem{\mi{fm}}_F$: set of valid feature selections}

===Guille:
$\sem{\mi{fm}}_F$: set of valid feature selections\\

\vspace{2mm}
===Rolf: I would suggest to switch the arguments:
\begin{itemize}
	\item $\fstype:\sem{\mi{fm}}_F \to (\com \to \{(\kw{snd},\kw{rcv})\}$
\end{itemize}
or
\begin{itemize}
	\item $\fstype:\sem{\mi{fm}}_F \to \textbf{St}_{\com}$
\end{itemize}
where $\textbf{St}_{\com}$ is the set of synchronisation type specifications over $\com$. 
This shows our idea to associate to each valid product a synchronisation type specification.

===end Rolf\\
\guille{I agree, it fits better.}

\stype with variability might delay the decision of which transitions and requirements 
are valid until compliance check. Now transitions can satisfy an \stype in some products 
and not in others. Same for requirements.
When building $\E$ from a \stype with variability, the only 
transitions we can discard for sure, are those that don't satisfy \stype in any product. 
Similar, we can discard requirements if they are not valid in any product.
This means we probably need \stype during compliance check and during projection.
An alternative would be to add extra restrictions (feature expressions) 
to transitions and requirements to explicitly say the products that satisfy that transition 
or requirement in terms of \stype.
There is a small draw with examples of both approaches here: 
\url{https://guillerminacledou586305.invisionapp.com/freehand/team-automata-examples-chSUnSRsh}

\subsection{Idea 1}
This alternative requires to pay attention to \stype during compliance and projection.

\vspace{2mm}
===Rolf: Yes, during projection we must then remove also those transitions which do not fit to the synchronisation type
specified by the product. But even then we would perhaps not get the desired commutative diagram. It seems that
the notion of valid transition would not really help, because of the existential quantifier.\\

\myparagraph{Valid transition in terms of \stype:}\\
A transition satisfies $\stype(a)$ if it satisfies $\stype(a)_p$ for some product $p$
% \begin{itemize}
% 	\item $q\ttr[\varphi]{(S,a,R)}q' \models \stype(a)_p = (\kw{s},\kw{r})
% 		~\bkw{if}~ p \models \varphi \bkw{ and } |S| \in \kw{s} \bkw{ and } |R| \in \kw{r}$
%   \item $q\ttr[\varphi]{(S,a,R)}q' \models \stype(a) 
% 		~\bkw{if}~ \exists_{p \in\sem{\fm}} ~\cdot~ q\ttr[\varphi]{(S,a,R)}q' \models \stype(a)_p$
% \end{itemize} 
(with alternative notation): 

\begin{align*}
	q\ttr[\varphi]{(S,a,R)}q' \models& \stype(a)_p &&~\bkw{if}~
	\left[
	\begin{array}{c}
		\Big[a\in\com \land \stype(a)_p = (s,r)\Big] ~\bkw{implies}~\\
		\Big[p \models \varphi \bkw{ and } |S| \in s \bkw{ and } |R| \in r\Big]
	\end{array}
	\right]
% \end{align*}	
% \begin{align*}
	\\
	q\ttr[\varphi]{(S,a,R)}q' \models& \stype 
	&&~\bkw{if}~ \exists_{p \in\sem{\fm}} ~\cdot~ q\ttr[\varphi]{(S,a,R)}q' \models \stype(a)_p 
\end{align*}

\myparagraph{Valid requirement in terms of \stype:}\\
A requirement is valid if it is valid for some product
% \[\begin{array}{l@{~~~}l}
% \rcp(J,a)@q\mshl{_{\varphi}} \text{ is \bkw{valid} for } \stype(a)_p = (\kw{s},\kw{r}) 
% 		&\bkw{if } p \models \varphi \bkw{ and } |J|\in \kw{s}  \bkw{ and } 
% 		\kw{r}.i_1{\color{red!80}{,\kw{r}.o_1}}\neq 0
% \\[2mm]
% \rcp(J,a)@q\mshl{_{\varphi}} \text{ is \bkw{valid} for } \stype(a) 
% 		&\bkw{if } \exists_{p\in\sem{\fm}} ~\cdot~ 
% 		\rcp(J,a)@q\mshl{_{\varphi}} \text{is \bkw{valid} for } \stype(a)_p 
% \\[2mm]
% \rsp(J,a)@q\mshl{_{\varphi}} \text{ is \bkw{valid} for } \stype(a)_p  = (\kw{s},\kw{r})
% 		&\bkw{if } p \models \varphi \bkw{ and } |J| \in \kw{r} \bkw{ and } 
% 		\kw{s}.o_1{\color{red!80}{,\kw{s}.i_1}}\neq 0 \bkw{ and}
% 		\\ &
% 		\text{ \sout{if $\forall_{j\in J}\cdot q_j$ has only inputs enabled}}
% \\[2mm]
% \rsp(J,a)@q\mshl{_{\varphi}} \text{ is \bkw{valid} for } \stype(a) 
% 		&\bkw{if } \exists_{p\in\sem{\fm}} ~\cdot~
% 		\rsp(J,a)@q\mshl{_{\varphi}} \text{ is \bkw{valid} for } \stype(a)_p 	
% \end{array}\]
(with alternative notation): 
\[\begin{array}{l@{~~~}l}
\rcp(J,a,\varphi) \models \stype(a)_p = ([s_1,s_2],[r_1,r_2]) 
		&\bkw{if } p \models \varphi \bkw{ and } |J|\in [s_1,s_2] \bkw{ and } 
		r_1{\color{red!80}{,s_1}}\neq 0
\\[2mm]
\rcp(J,a,\varphi) \models \stype 
		&\bkw{if } \exists_{p\in\sem{\fm}} ~\cdot~ 
		\rcp(J,a,\varphi) \models \stype(a)_p 
\\[2mm]
\rsp(J,a,\varphi) \models \stype(a)_p  = ([s_1,s_2],[r_1,r_2]) 
		&\bkw{if } p \models \varphi \bkw{ and } |J| \in [r_1,r_2] \bkw{ and } 
		s_1{\color{red!80}{,r_1}}\neq 0 
\\[2mm]
\rsp(J,a,\varphi)\models\stype 
		&\bkw{if } \exists_{p\in\sem{\fm}} ~\cdot~
		\rsp(J,a,\varphi)\models\stype(a)_p 	
\end{array}\]

\subsection{Idea 2}
To get rid of \stype earlier.

\myparagraph{Valid transition in terms of \stype:} same as idea 1

\myparagraph{Extended $\gamma$ for $\E(\stype)$:}

===Rolf:
You may write $\stype(\gamma)$ following the notation from above for $\stype(E)$.

\begin{align*}
	\gamma_{\E(\stype)}(t) = \ifcond{
		\begin{array}{l@{~~~}l}
			\gamma(t) & t.a\in \Sigma \setminus \com \\
			\gamma(t)\land \kw{fe}(P) & t.a\in\com ~\bkw{and}~ P = \{p\in\sem{\fm} ~|~ t\models \stype(a)_p\}
		\end{array}
	}
\end{align*} 
For $P$ a set of feature selections, $\kw{fe}(P) = \bigvee_{p\in P} (\bigwedge_{f\in p} f)$, \ie 
a feature expression capturing the logic OR of each valid feature selection $p\in P$.
In this case, a feature expression capturing the products in which $t$ satisfies \stype.

\vspace{2mm}
===Rolf:
We should remark that $ \bigvee_{p\in \emptyset} ... = \bot$.\\
I suggest to change the formula  $\kw{fe}(P)$ above to $\kw{fe}(P) = \bigvee_{p\in P} \kw{fe}(p)$ 
using the macro $\kw{fe}(p) = (\bigwedge_{f\in p} f) \wedge  (\bigwedge_{f\notin p} \neg f) $.
The current formulation is not quite correct, I think, because we need negations for the features not in $p$.
Otherwise, having a product $p = \{f\} \in P$, the formula  $f$ could also be satisfied by other valid products
like $q=\{f,g\}$ such that $\stype(a)_p$ and $\stype(a)_q$ do not fit together, i.e. $q \notin P$.
Then, projecting the transition $t$ w.r.t. product $q$ would give a result that cannot be obtained
in the ETA team automaton. 
Thus the commuting diagram (Theorem~\ref{thm:commuting}) would not hold anymore for $q$.
It's quite subtle, indeed.
\\\guille{I agree, indeed, the previous enconding of a products as a feature expression was wrong.}

\myparagraph{Valid requirement in terms of \stype:} same as idea 1

\myparagraph{Requirements generated by \stype in a state $q$: }\\

% Let $\kw{prod}(\rcp(a,J)@q\mshl{_{\varphi}}) = 
% 	\{p\in\sem{\fm} ~|~ \rcp(a,J)@q\mshl{_{\varphi}} ~\bkw{valid}~\text{for}~\stype(a)_p\}$, 
% be the set of all products in which the requirement is valid. 
Let $\kw{prod}(c) = 
	\{p\in\sem{\fm} ~|~ c\models\stype(c.\kw{act})_p\}$, 
be the set of all products in which the requirement $c \in (\rcp@q ~\uplus~ \rsp@q)$ is valid.

% \begin{itemize}
% 	\item $\rcp@q$:\\
% 		$\bigwedge \{\rcp(J,a)@q\mshl{_{\varphi\land\kw{fe}(P)}} ~|~ 
% 			a\in\com, 
% 			P = \kw{prod}(\rcp(J,a)@q\mshl{_{\varphi}}), 
% 			P\neq\emptyset\}$
% 	\item $\rsp@q$: \\
% 	$\bigvee \{\rsp(J,a)@q\mshl{_{\bkw{in}(J)_q\land\varphi\land\kw{fe}(P)}} ~|~ 
% 			a\in\com, 
% 			P=\kw{prod}(\rsp(J,a)@q\mshl{_{\varphi}}),
% 			P \neq\emptyset\}$	
% \end{itemize}
\begin{itemize}
	\item $\stype(\rcp@q)$:\\
		$\bigwedge \{\rcp(J,a,\mshl{\varphi\land\kw{fe}(P)}) ~~~~~~~~~~~~~~|~ 
			a\in\com,~ 
			P = \kw{prod}(\rcp(J,a,\varphi)@q), ~
			P\neq\emptyset\}$
	\item $\stype(\rsp@q)$: \\
	$\bigvee \{\rsp(J,a,\mshl{\varphi\land\bkw{in}(J)_q\land\kw{fe}(P)}) ~|~ 
			a\in\com, ~
			P=\kw{prod}(\rsp(J,a,\varphi)@q),~
			P \neq\emptyset\}$	
\end{itemize}
where $\mshl{\bkw{in}(J)_q}= \kw{fe}(\bigvee\{p~|~ p\in\sem{\fm}, \forall_{j\in J} \cdot q_{j\proj_p} 
	\text{ has only inputs enabled}\})$ with ($q_{j\proj_p}\in A_j\proj_p$), 
	\ie $\mshl{\bkw{in}(J)_q}$ are the products in which all $J$ are only input enabled at $q$.

\input{ex2}
